# Supplementary material for: Batched Stochastic Bayesian Optimization via Combinatorial Constraints Design
Source: arXiv:1904.08102 source file (2019-04-17)
Supplement: Supplementary file 1 [file appendix-notes.tex]

\newpage
\section{Notes}
\begin{itemize}
  % \item When selecting the $t$-th batch, some entries are already filled in -- still DS optimization?
\item Can we generalize the problem to other domains?
  \begin{itemize}
  \item Actions: constraints/ rules/ formal specifications
  \item Utility: joint utility of the samples generated under the specified constraints
  \end{itemize}
\end{itemize}

%%% Local Variables:
%%% mode: latex
%%% TeX-master: "main"
%%% End:
